# Supplementary material for: Sub-100-fs formation of dark excitons in monolayer WS2
Source: arXiv:2403.08390 source file (2024-08-06)
Supplement: Supplementary file 1 [file supplementary.pdf]

# Supplementary material to: "Sub-100-fs formation of dark excitons in monolayer WS<sub>2</sub>"

Pavel V. Kolesnichenko,<sup>\*,†,‡</sup> Lukas Wittenbecher,<sup>¶</sup> Qianhui Zhang,<sup>⊥</sup> Run Yan Teh,<sup>#</sup> Chandni Babu,<sup>§</sup> Michael S. Fuhrer,<sup>@,△</sup> Anders Mikkelsen,<sup>¶</sup> and Donatas Zigmantas<sup>\*,§</sup>

<sup>†</sup>*Institute of Physical Chemistry, Heidelberg University, 69120, Heidelberg, Germany*

<sup>‡</sup>*Institute for Molecular Systems, Engineering and Advanced Materials, Heidelberg University, 69120, Heidelberg, Germany*

<sup>¶</sup>*Department of Physics, Lund University, Box 118, 221 00 Lund, Sweden*

<sup>§</sup>*Division of Chemical Physics, Lund University, P.O. Box 124, 221 00 Lund, Sweden*

<sup>||</sup>*NanoLund, P.O. Box 124, 221 00 Lund, Sweden*

<sup>⊥</sup>*Department of Civil Engineering, Monash University, Melbourne, Victoria 3800, Australia*

<sup>#</sup>*Centre for Quantum Science and Technology Theory, Swinburne University of Technology, Melbourne, Victoria 3122, Australia*

<sup>@</sup>*School of Physics and Astronomy, Monash University, Melbourne, Victoria 3800, Australia*

<sup>△</sup>*ARC Centre of Excellence in Future Low-Energy Electronics Technologies, Monash University, Melbourne, Victoria 3800 Australia*

E-mail: pavel.kolesnichenko@alumni.uni-heidelberg.de; donatas.zigmantas@chemphys.lu.se

## S1. Pulse spectra and time-resolution of TR-PEEM

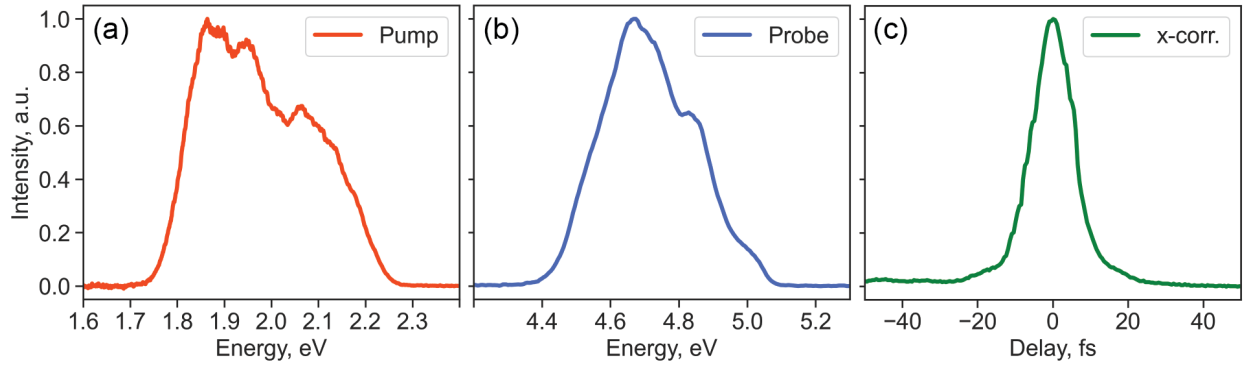

Figure S1: (a) Pump and (b) probe spectra, and (c) temporal cross-correlation (x-corr.) of pump and probe pulses measured via pump-induced transient-grating gate in a thin fused silica plate.<sup>1</sup> The x-corr. was measured in front of the PEEM's input window taking the window material into account. The fwhm of x-corr. profile is 13.4 fs defining temporal resolution of the TR-PEEM apparatus.

## S2. Spatial resolution of TR-PEEM

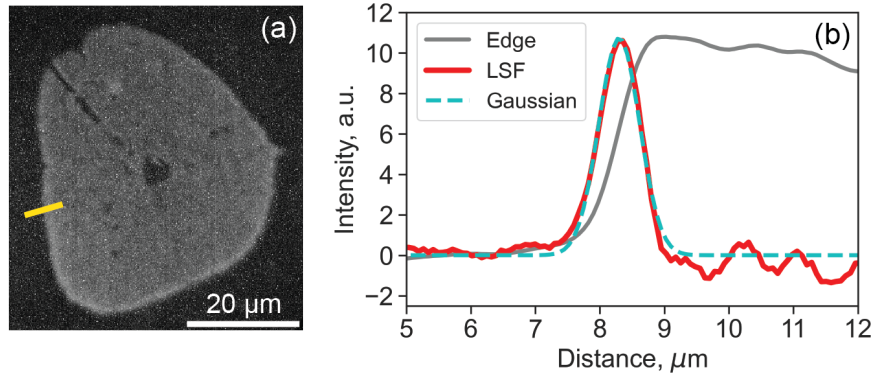

Figure S2: (a) Monolayer WS<sub>2</sub> flake imaged via a mercury lamp. (b) Edge profile (grey) taken along the yellow line indicated in (a), line spread function (LSF, red) of the edge profile, and a Gaussian fit to LSF with fwhm of 74.6 nm defining spatial resolution of the TR-PEEM apparatus.

### S3. Pump-induced excitation and photoemission

Table S1: Pump fluences and corresponding carrier excitation densities.

|                                              |      |      |      |      |
|----------------------------------------------|------|------|------|------|
| Pump fluence, $nJ/cm^2$                      | 8    | 17   | 34   | 136  |
| Excitation density, $10^{11} \times cm^{-2}$ | 0.52 | 1.05 | 2.12 | 8.49 |

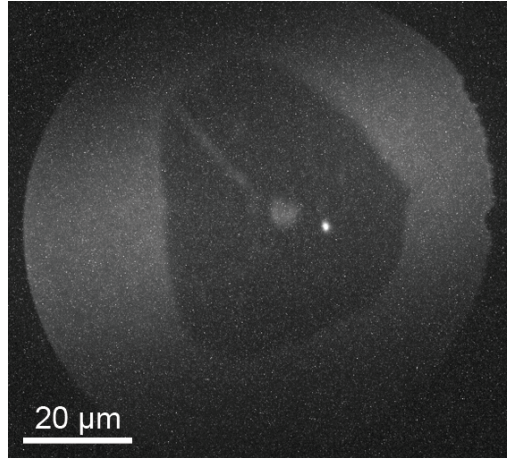

Figure S3: A photoemission image of the  $WS_2$  monolayer flake obtained using  $136 \text{ nJ}/cm^{-2}$  pump pulses (with probe pulses blocked).

### S4. Monolayer-specific dynamics

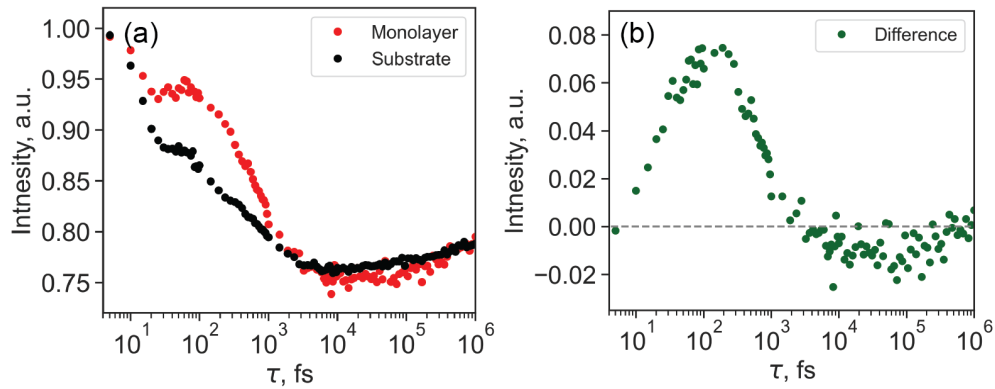

Figure S4: (a) Normalization of raw pump-probe traces obtained from  $WS_2$  monolayer interior and substrate. (b) Difference (also Figure 2a of the main text) between the pump-probe traces in (a). Pump fluence was  $34 \text{ nJ}/cm^2$ .

The two spectra were pinned at 0 fs and 1 ns delays (Figure S4a) and subtracted (Figure S4b). This procedure naturally suppresses the effects from pulse overlap including coherent exciton population signal.

## S5. Fittings of pump-probe traces

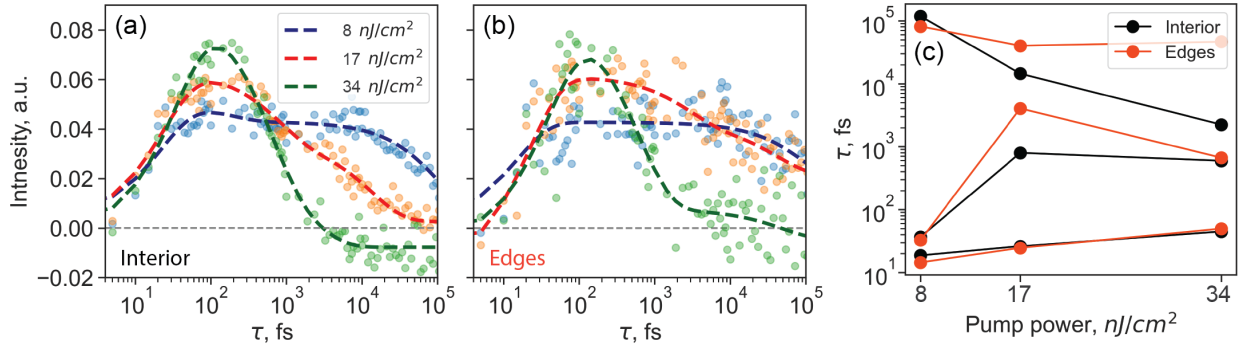

Figure S5: Fittings of the pump-probe traces shown in Figure 2b of the main text.

Table S2: Extracted time-constants for the three pump fluences (interior of the flake)

|                   | 8 $nJ/cm^2$ | 17 $nJ/cm^2$ | 34 $nJ/cm^2$ |
|-------------------|-------------|--------------|--------------|
| $\tau_{rise}, fs$ | 18.7        | 26.3         | 45.1         |
| $\tau_1, fs$      | 36.9        | 797          | 596          |
| $\tau_2, ps$      | 118.2       | 14.5         | 2.2          |

Table S3: Extracted time-constants for the three pump fluences (flake's edges)

|                   | 8 $nJ/cm^2$ | 17 $nJ/cm^2$ | 34 $nJ/cm^2$ |
|-------------------|-------------|--------------|--------------|
| $\tau_{rise}, fs$ | 14.5        | 24.6         | 50.0         |
| $\tau_1, fs$      | 32.7        | 2747         | 624          |
| $\tau_2, ps$      | 81.6        | 40.2         | 46.6         |

## S6. Photoemission contrast drop for higher pump fluences

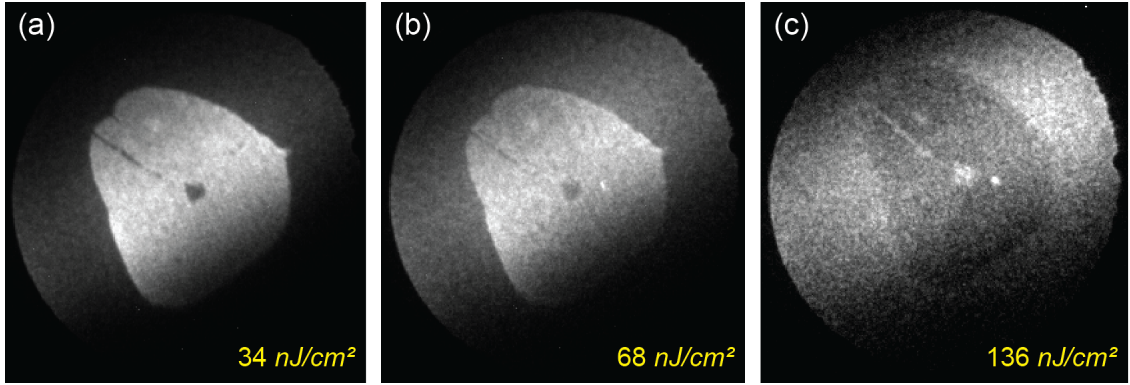

Figure S6: Photoemission at 7 ps pump-probe delay for three pump fluences of (a)  $34 \text{ nJ/cm}^2$ , (b)  $68 \text{ nJ/cm}^2$ , and (c)  $136 \text{ nJ/cm}^2$ . For higher fluences photoemission contrast from the flake becomes lower.

## S7. Fitting with two rise-and-decay signals

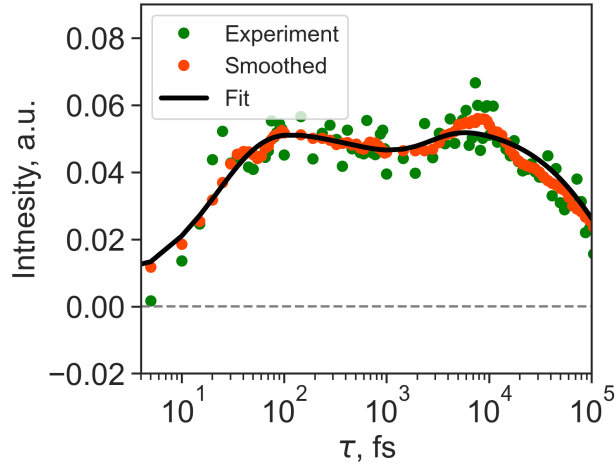

Figure S7: Fitting with a model (Eq. (S1)) accounting for two rise-and-decay signals. Pump fluence is  $8 \text{ nJ/cm}^2$ .

Extracted rise time-constants are  $\tau_{rise,1} \sim 23.7 \text{ fs}$  and  $\tau_{rise,2} \sim 1.1 \text{ ps}$  comparable to

previously reported values of dark-exciton<sup>2,3</sup> and trion formation.<sup>4</sup>

$$I = \left( (1 - a_{rise,1} e^{-\frac{\tau - \tau_{0,1}}{\tau_{rise,1}}}) \cdot a_1 e^{-\frac{\tau - \tau_{0,1}}{\tau_1}} + (1 - a_{rise,2} e^{-\frac{\tau - \tau_{0,2}}{\tau_{rise,2}}}) \cdot a_2 e^{-\frac{\tau - \tau_{0,2}}{\tau_2}} + a_0 \right) \cdot H(\tau - \tau_0) \quad (\text{S1})$$

## References

1. Bruder, L.; Wittenbecher, L.; Kolesnichenko, P. V.; Zigmantas, D. Generation and compression of 10-fs deep ultraviolet pulses at high repetition rate using standard optics. *Optics Express* **2021**, *29*, 25593.
2. Wang, L.; Xu, C.; Li, M.-Y.; Li, L.-J.; Loh, Z.-H. Unraveling Spatially Heterogeneous Ultrafast Carrier Dynamics of Single-Layer WSe<sub>2</sub> by Femtosecond Time-Resolved Photoemission Electron Microscopy. *Nano Letters* **2018**, *18*, 5172–5178.
3. Wallauer, R.; Perea-Causin, R.; Münster, L.; Zajusch, S.; Brem, S.; Gädde, J.; Tanimura, K.; Lin, K.-Q.; Huber, R.; Malic, E.; Höfer, U. Momentum-Resolved Observation of Exciton Formation Dynamics in Monolayer WS<sub>2</sub>. *Nano Letters* **2021**, *21*, 5867–5873.
4. Singh, A.; Moody, G.; Tran, K.; Scott, M. E.; Overbeck, V.; Berghäuser, G.; Schaibley, J.; Seifert, E. J.; Pleskot, D.; Gabor, N. M.; Yan, J.; Mandrus, D. G.; Richter, M.; Malic, E.; Xu, X.; Li, X. Trion formation dynamics in monolayer transition metal dichalcogenides. *Physical Review B* **2016**, *93*, 041401(R).
